# Supplementary material for: Producing radiologist-quality reports for interpretable artificial intelligence
Source: arXiv:1806.00340 ancillary file (2018-06-01)
Supplement: Supplementary file 1 [file supplementary_file.pdf]

---

## Supplement: Producing radiologist-quality reports for interpretable artificial intelligence.

---

**William Gale\*, Gustavo Carneiro**

School of Computer Science

The University of Adelaide

Adelaide, SA 5000

will@gale.com

gustavo.carneiro@adelaide.edu.au

**Luke Oakden-Rayner\*, Lyle J. Palmer**

School of Public Health

The University of Adelaide

Adelaide, SA 5000

{luke.oakden-rayner, lyle.palmer}

@adelaide.edu.au

**Andrew P. Bradley**

Faculty of Science and Engineering

Queensland University of Technology

Brisbane, QLD 4001

a6.bradley@qut.edu.au

### Supplementary Material

In this supplementary material, we present more randomly selected examples of fractures, saliency maps, and both the original report descriptions and the generated text explanations in Figures 1–3.

### References

- [1] Smilkov, D., Thorat, N., Kim, B., Viégas, F., Wattenberg, M.: Smoothgrad: removing noise by adding noise. arXiv preprint arXiv:1706.03825 (2017)

---

\* These authors contributed equally to the work

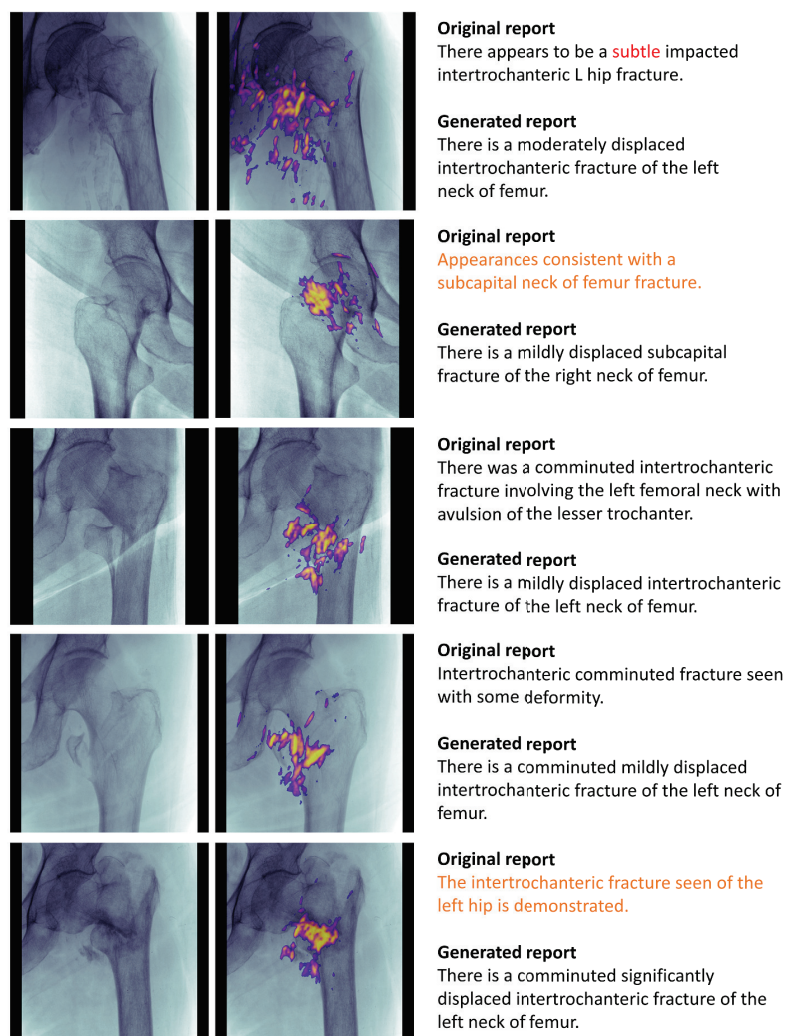

**Figure 1:** Randomly selected examples, showing the original image, the SmoothGrad saliency map [1], the original report description, and the generated sentence. Orange highlights indicate that the sentence does not appropriately characterise the fracture. Red highlights indicate that the radiologist thought an alternative descriptive term was more appropriate.

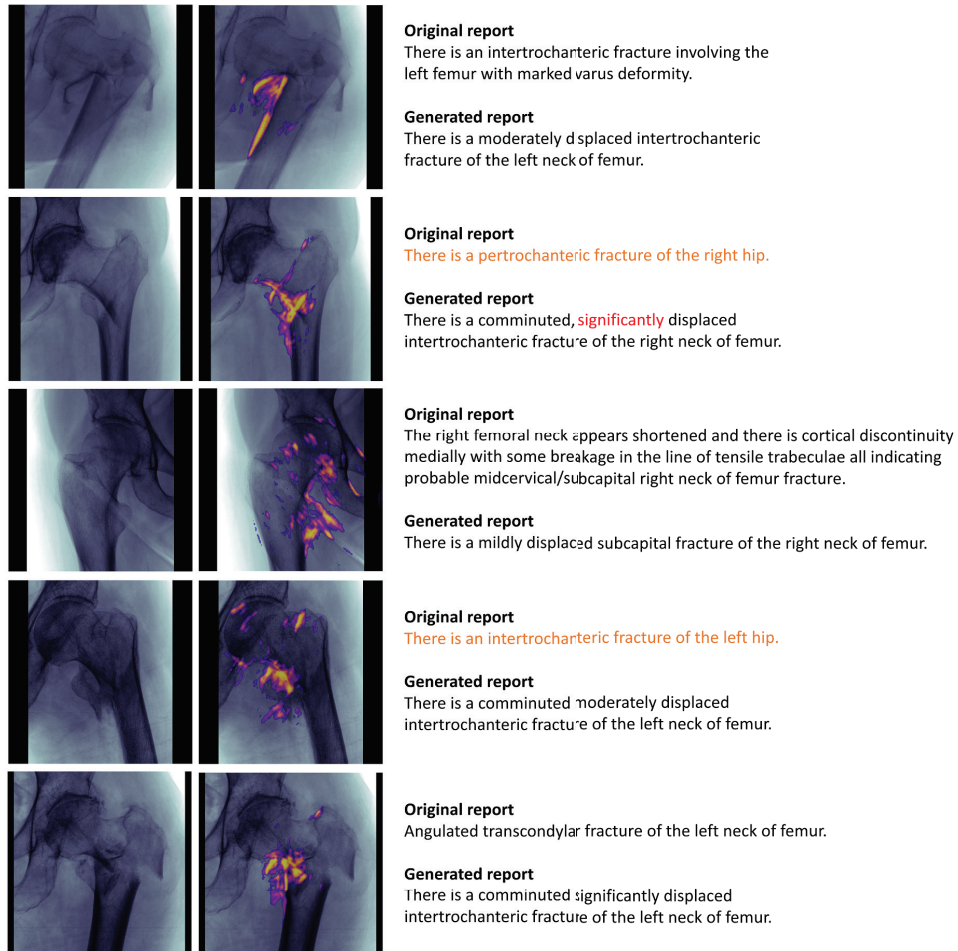

**Figure 2:** Randomly selected examples, showing the original image, the SmoothGrad saliency map [1], the original report description, and the generated sentence. Orange highlights indicate that the sentence does not appropriately characterise the fracture. Red highlights indicate that the radiologist thought an alternative descriptive term was more appropriate.

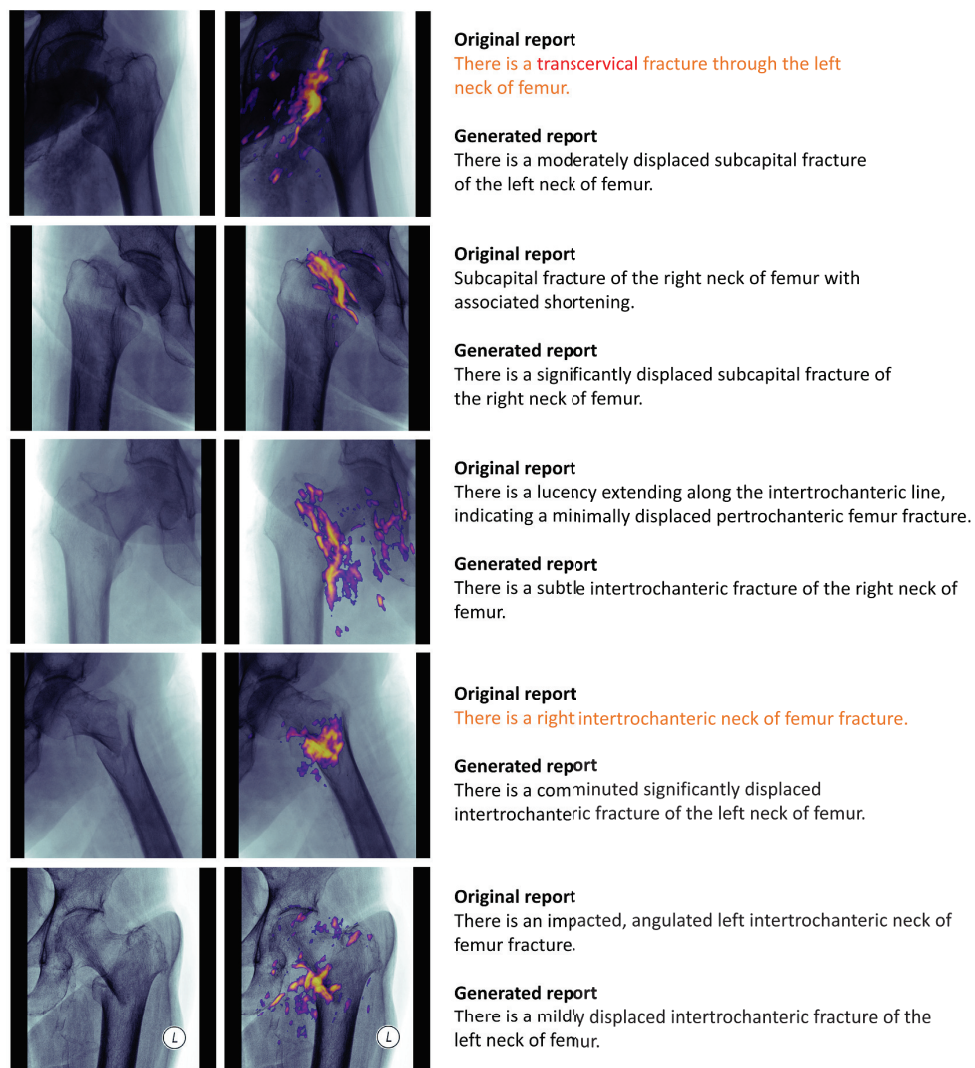

**Figure 3:** Randomly selected examples, showing the original image, the SmoothGrad saliency map [1], the original report description, and the generated sentence. Orange highlights indicate that the sentence does not appropriately characterise the fracture. Red highlights indicate that the radiologist thought an alternative descriptive term was more appropriate.
